# Supplementary material for: What's Behind the Couch? Directed Ray Distance Functions (DRDF) for 3D Scene Reconstruction
Source: arXiv:2112.04481 source file (2022-04-04)
Supplement: Supplementary file 1 [file supp_decoding.tex]

\dfnote{Not sure this goes here. This can almost certainly fit in the main paper when explaining the baselines }

We report the design decisions used in the baselines and our method. Throughout, let $S$ denote a set of surface intersections along a ray.

\parnobf{Unsigned Distance Function (UDF)}

The UDF $\min_{s \in S} |z-s|$ still has a minimum and derivative sign-change at the intersection under expectation. We aim to use ths.

\parnoit{Direct Thresholding} We look for the zero-crossings of $\hat{d}_U(z;s) - \tau$ for varying $\tau$.

\parnoit{Gradient Zero-Crossing} Since the expected UDF still changes its derivative's sign at the intersection, we compute numerical derivatives and locate zero-crossings.

\parnoit{Thresholding with Non-Maximum Suppression} \dfnote{what}

\parnobf{Sign Agnostic Learning (SAL)} Since SAL produces a signed distance function, we look for zero-crossings.

\parnobf{Occupancy Function (OF)}
The OF $d_O = (\min_{s \in S} |z-s|) < r$ has a binarization parameter, namely the radius $r$. We optimize $r$ on the validation set (for $1$m, $0.5$m, $0.25$m, $0.1$m). 

\parnoit{Thresholding} Following \cite{saito2019pifu}, we find zero-crossings of $\hat{d}_O(z;s)-0.5$ for the predicted distance $\hat{d}_O$. However, since these include both entrances and exits to the $r$-ball at the intersection, we only include positive-to-negative zero-crossings to avoid repeated phantom intersections.

\parnoit{Peak-Finding} Since the expected function still has a peak at the intersection, we find peaks using \dfnote{what}.

\parnoit{Averaging Entrances and Exits} The first thresholding approach induces a bias in the predictions: the intersections are all systematic underestimates. We correct this by pairing adjacent positive-to-negative and negative-to-positive zero-crossings that could represent the adjacent zero-crossings of an intersection (correct order, distance), and average them.

\parnobf{Directed Ray Distance Function (DRDF)}
For the DRDF, we simply look for zero-crossings.
