# Supplementary material for: What's Behind the Couch? Directed Ray Distance Functions (DRDF) for 3D Scene Reconstruction
Source: arXiv:2112.04481 source file (2022-04-04)
Supplement: Supplementary file 2 [file interactive_demo.tex]

\subsection{Approach Overview}
We show an overview of the approach in \texttt{approach\_overview.webm}. It discusses the challenges in designing a single image to 3D system trained on real 3D scene data and presents our approach briefly.
% $\bullet$ . We describe the overview of our approach in a {\it 5 minute} video. We discuss the challenges and our approach from the paper.\\
\subsection{Video Results}
\label{sec:video}
We provide {\it three} video files with results from our models. These videos show the outputs of our model
and compare them to the ground truth and baselines by showing salient features at different instances in video frames. All the videos files are best viewed a web-browser\\
\noindent
$\bullet$ \texttt{result\_videos/main\_paper.mp4}. Shows the qualitative results from Fig 6, and Fig 7 of the main paper in order of their appearance. We highlight salient regions our model similar to the zoom-ins in the main paper to qualitatively compare the outputs. The first part of the video compares the DRDF outputs with ground truth and the second part of the video compares against various baselines. This video contains {\it all} the qualitative examples in the main paper.\\
$\bullet$ \texttt{result\_videos/additional.mp4}. This video shows additional qualitative examples in addition to the main qualitative examples shown. It is also divided into two parts where the first part compares against ground truth while the second part compares against outputs of other baseline methods.\\
$\bullet$ \texttt{result\_videos/supp\_qual.mp4}. This video shows six samples from the qualitative figures shown in the supplemental in \figref{fig:matterport_novel}, \ref{fig:threedf_novel}, \ref{fig:scannet_novel} (2 samples from each dataset) and compares the outputs against the ground truth.
\begin{figure}
    \centering
    \includegraphics[width=0.8\textwidth]{suppfigures/video.jpg}
    \caption{{\bf Qualitative Video.} Screen Capture from \texttt{main\_paper.mp4}. Our video shows model outputs and a highlight box (red/black) describing regions of interest and salient differences between methods. Our supplementary contains three videos of results each showcasing a different set of examples. a) \texttt{main\_paper.mp4} has all the results from the main paper and we highly encourage watching this. b) \texttt{additional.mp4} has more result showcasing performance with respect to other baselines, and ground-truth c) \texttt{supp\_qual.mp4} has video results for samples in the supplementary PDF}. 
 \end{figure}

\subsection{Interactive Demo}
\label{sec:interactive_demo}
We provide three outputs of DRDF from the main paper and  embed them inside the HTML as an interactive demo to qualitatively assess our outputs and compare against the GT. The demo allows us to view the outputs from the given input image (left most column on the demo) and compare with GT(middle column on the demo) with the prediction (right most column on the demo)
Inside the folder \texttt{interactive\_demo} is a file \texttt{model\_vis.html}. Open this file in a web browser (best viewed in Google Chrome or Firefox) to see the interactive demo of the output from our model.
\begin{figure}
    \centering
    \includegraphics[width=0.8\textwidth]{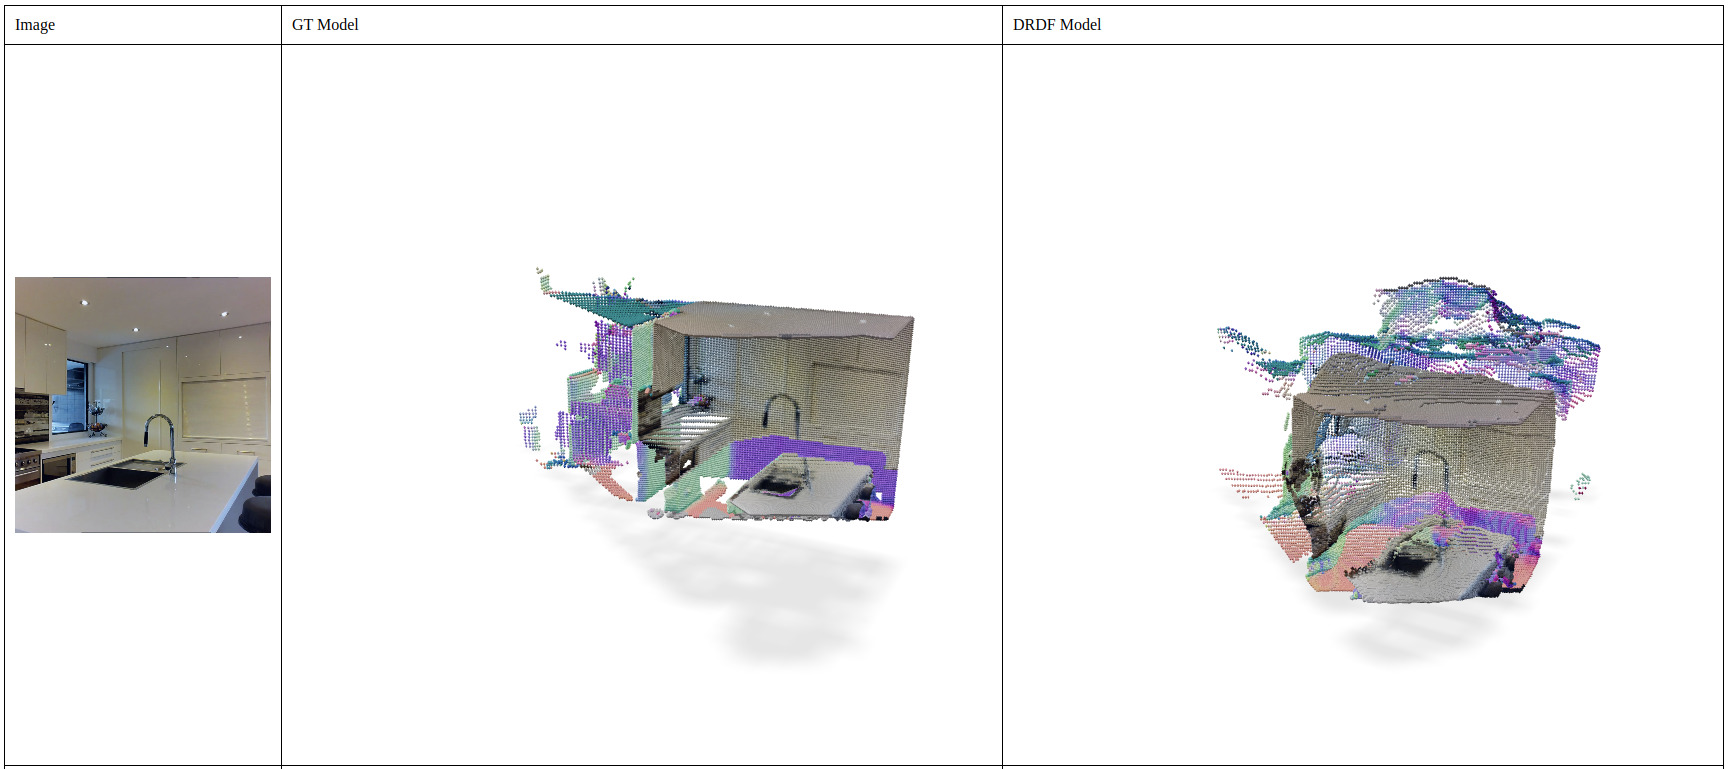}
    \caption{{\bf Interactive Demo.} Screen Capture of interactive demo. We present an interactive demo of selected outputs from the main paper, allowing explorations from more camera view-points not explored completely in the video trajectory. Please open the \texttt{model\_vis.html} in your web-browser (works best with Google Chrome and Firefox).}
\end{figure}
