# Supplementary material for: What's Behind the Couch? Directed Ray Distance Functions (DRDF) for 3D Scene Reconstruction
Source: arXiv:2112.04481 source file (2022-04-04)
Supplement: Supplementary file 3 [file supp_baselines.tex]

One of the key challenges of

\parnobf{Unsigned Distance Function}

\parnobf{Sign-Agnostic Loss}

\parnobf{Occupancy Function}
